# Supplementary material for: Reconfigurable Interaction for MAS Modelling
Source: arXiv:1906.10793 source file (2020-02-19)
Supplement: Supplementary file 1 [file appendix1.tex]

% !TEX root = ../main.tex
\section{Proofs}\label{sec:appendix}

In this appendix, we report the proofs of Lemma~\ref{lem:dlts=ds}, 
Theorem~\ref{thm:satisfiability} and Theorem~\ref{thm:modcheck} that are 
omitted from the main paper due to space limitation.

\begin{lemma}
	The traces of a system composed of a set of agents $\{A_{\id}\}_{\id}$ are 
	the paths of the induced doubly-labeled transition system.
	%  Given a set of agents $\{A_{\id}\}_{\id}$ their system traces
	%  are the paths of the induced doubly-labeled transition system.
\end{lemma}

\begin{proof}%[Proof of Lemma~\ref{lem:dlts=ds}]
The conditions on the sender in the transition system are that the send
transition of the sender hold corresponding to the conjunct
$\pfunc{\trans}{s}{k}$ for the sender $k$.
The conditions on the receivers in the transition system correspond to
the three different disjuncts in the definition of the system trance
(and $\rho$ of the discrete system):
\begin{itemize}
\item
  the receive transition of the receiver holds
  ($\pfunc{\trans}{r}{j}$), the receiver is interested in the channel
  ($\pfunc{g}{r}{j'}$), and by quantifying the values of the common
  variables separately for each $j\neq k$ and requiring $f_j$ and
  $\pfunc{g}{s}{k}$ effectively we require that the predicate obtained
  from $\pfunc{g}{s}{k}$, when translated to local variables of
  component $j$ holds over $j$'s copy of the local copies of the
  common variables.
\item
  the receiver is not interested in the channel ($\neg
  \pfunc{g}{r}{j}$), which means that the component $j$ does not
  change its local state variables.
\item
  only in a broadcast, the receiver is not an intended recipient of
  the message ($\neg \pfunc{g}{s}{k}$) and hence does not change its
  local state variables.
\end{itemize}
\end{proof}

\begin{theorem}
	The satisfiability problem of \ltal is \pspace-complete with respect to 
	$\size{\phi}$, $\size{\sysvar},\ \size{\sdat},\ \log{\size{\schan}},\ 
	\log{\size{K}}$ and \expspace with respect to $\size{\scv}$. 
\end{theorem}

\begin{proof}
	
	By Corollary~\ref{cor:1}, for a given \ltal formula $\phi$, there exists a 
	nondeterministic B\"{u}chi automaton $A_{\phi}$ accepting all and only the 
	computations satisfying $\phi$, whose state-space $Q$ is of size exponential 
	in the length of $\phi$, the state-alphabet $\Sigma$ is exponential in the 
	number of local variables, and the message alphabet $M$ is linear in the 
	number of channels and the number of agents, singly exponential in the number 
	of data variables, and doubly exponential in the the number of common 
	variables.
	Thus, the satisfiability problem of \ltal reduces to the emptiness problem of 
	the automaton $A_{\phi}$, whose complexity is \nlogspace.
	Observe that, again by Corollary~\ref{cor:1}, the construction and emptiness 
	check of $A_{\phi}$ can be done on-the-fly, thus providing a satisfiability 
	procedure that is \pspace with respect to $\size{\phi}$, $\size{\sysvar}$, 
	$\size{\sdat}$, $\log{\size{\schan}}$, $\log{\size{K}}$ and \expspace with 
	respect to $\size{\scv}$.
	
	The lower bound follows from the satisfiability of \ltl, that can be regarded 
	as an \ltal formula with no occurrences of common variables.

%By Corollary~\ref{cor:1}, given a formula $\phi$, we can construct a
%B\"uchi automaton $A_n$ of size $\size{Q_n}.\size{\delta_n}$ that
%accepts precisely the computations that satisfy $\phi$. Thus, $\phi$
%is satisfiable iff $A_n$ is nonempty. The satisfiability problem is
%reduced to the nonemptiness of $A_n$. The nonemptiness of a B\"uchi
%automaton is tested in nondeterministic logarithmic space and we get a
%polynomial space algorithm with respect to $\size{\phi}$,
%$\size{\sysvar},\ \size{\sdat},\ \log{\size{\schan}},\ \log{\size{K}}$
%and EXPSPACE with respect to $\size{\scv}$. The algorithm constructs
%$A_n$ on-the-fly. The hardness argument~\cite{sistlac85} can be proved
%by the fact that any PSPACE-hard problem can be reduced to the
%satisfiability problem.   
\end{proof}

\begin{theorem}
	The model-checking problem of \ltal is \pspace-complete with respect to 
	$\size{Sys}$, $\size{\phi}$, $\size{\sysvar},\ \size{\sdat},\ 
	\log{\size{\schan}},\\ \log{\size{K}}$ and \expspace with respect to 
	$\size{\scv}$. 
\end{theorem}

\begin{proof}
	Consider a discrete system $Sys = \conf{\sysvar, \rho, \theta}$ and a set of 
	assertions on state variables $\sysvar$, on $\schan,\ {\sdat},\ K$, and on 
	$cv_1, \dots, cv_n$.
	We assume $\rho$ to be total and then we can construct an automaton 
	$A_{Sys} = \conf{S,\Sigma, M, S_0, \delta_s, S}$ such that the set of states 
	$S$ is 
	the set of possible interpretations of the variables in $\sysvar$.
	The set of initial states $S_0$ is the set of states $s$ such that $s\models 
	\theta$, i.e., $S_0=\set{s\models {\theta}}$, $\Sigma=\Exp{\sysvar}$, and  
	$M=\schan\times\Exp{\sdat}\times K\times \dexp{\scv}$.
	We have that $\delta_s(s,\sigma,m)=\set{s': \tuple{s,\sigma,m,s'}\models 
	\rho}$ and $\emptyset$ otherwise.
	The number of states in the transition system may be exponentially larger 
	than the description of $Sys$.
	
	$Sys$ satisfies $\phi$ if, and only if, all the computations of $Sys$ satisfy 
	$\phi$, thus $\lang{A_{Sys}}\subseteq \lang{A_{\phi}}$.
	This is equivalent to check $\lang{A_{Sys}}\cap\lang{A_{\neg 
	\phi}}=\emptyset$. 
	Since our formulas are in positive normal form, $\neg\phi$ can be obtained 
	from $\phi$ by $\overline{\phi}$.
	By Corollary~\ref{cor:1}, we have that $A_{\neg\phi}$ has 
	$\Exp{\bigo{\size{\phi}}}$ states and $\size{A_{\neg\phi}}$ is in
	$\bigo{\size{\schan}.\size{K}.\Exp{\size{\phi}+\size{\sysvar}+\size{\sdat}+\Exp{\size{\scv}}}}$.
	The model checking problem can be reduced to the nonemptiness problem of the 
	intersection of $A_{s}$ and $A_{\neg\phi}$.
	Since all states in $A_{s}$ are accepting, the construction of 
	$A_{s,\neg\phi}$ is the product of $A_{s}$ with $A_{\neg\phi}$. We have that 
	$A_{s,\neg\phi}$ has $\Exp{\bigo{\size{Sys}+\size{\phi}}}$ states.
	Hence, $\size{A_{s, \neg\phi}}$ is in 
	$$\bigo{\size{\schan} \cdot \size{K} 
	\cdot \Exp{\size{\phi} + \size{Sys} + \size{\sysvar} + \size{\sdat} + 
	\Exp{\size{\scv}}}}\text{.}$$
	\noindent We have that $A_{s,\neg\phi}$ can be constructed on-the-fly and a 
	membership 
	in \pspace with respect to $\size{Sys}$, $\size{\phi}$, $\size{\sysvar}$, 
	$\size{\sdat}$, $\log{\size{\schan}}$, $\log{\size{K}}$ and a membership in 
	\expspace with respect to $\size{\scv}$ follow from the membership in 
	NLOGSPACE of the nonemptiness problem for NBW.
	Checking that $Sys\models\phi$ is in
	
	$$\bigo{\log\size{\schan} + \log\size{K} 
	+ {\size{\phi} + \size{Sys} + \size{\sysvar} + \size{\sdat} + 
	\Exp{\size{\scv}}}}\text{.}$$

	The lower bound follows from the hardness of \ltl model 
	checking.~\cite{sistlac85}.
\end{proof}
