# Supplementary material for: Reconfigurable Interaction for MAS Modelling
Source: arXiv:1906.10793 source file (2020-02-19)
Supplement: Supplementary file 2 [file appendix.tex]

% !TEX root = ../main.tex
\section{Appendix}\label{sec:appendix}

\begin{proof}[Proof of Lemma~\ref{lem:dlts=ds}]
The conditions on the sender in the transition system are that the send
transition of the sender hold corresponding to the conjunct
$\pfunc{\trans}{s}{k}$ for the sender $k$.
The conditions on the receivers in the transition system correspond to
the three different disjuncts in the definition of the system trance
(and $\rho$ of the discrete system):
\begin{itemize}
\item
  the receive transition of the receiver holds
  ($\pfunc{\trans}{r}{j}$), the receiver is interested in the channel
  ($\pfunc{g}{r}{j'}$), and by quantifying the values of the common
  variables separately for each $j\neq k$ and requiring $f_j$ and
  $\pfunc{g}{s}{k}$ effectively we require that the predicate obtained
  from $\pfunc{g}{s}{k}$, when translated to local variables of
  component $j$ holds over $j$'s copy of the local copies of the
  common variables.
\item
  the receiver is not interested in the channel ($\neg
  \pfunc{g}{r}{j}$), which means that the component $j$ does not
  change its local state variables.
\item
  only in a broadcast, the receiver is not an intended recipient of
  the message ($\neg \pfunc{g}{s}{k}$) and hence does not change its
  local state variables.
\end{itemize}
\end{proof}

%\lowerboundproof
